# Supplementary material for: ClearBuds: Wireless Binaural Earbuds for Learning-Based Speech Enhancement
Source: arXiv:2206.13611 source file (2022-06-27)
Supplement: Supplementary file 1 [file 10-appendix.tex]

\appendix

\section{Appendix}

\begin{figure}[h]
\vskip -0.1in
\centering
\includegraphics[width=0.7\linewidth]{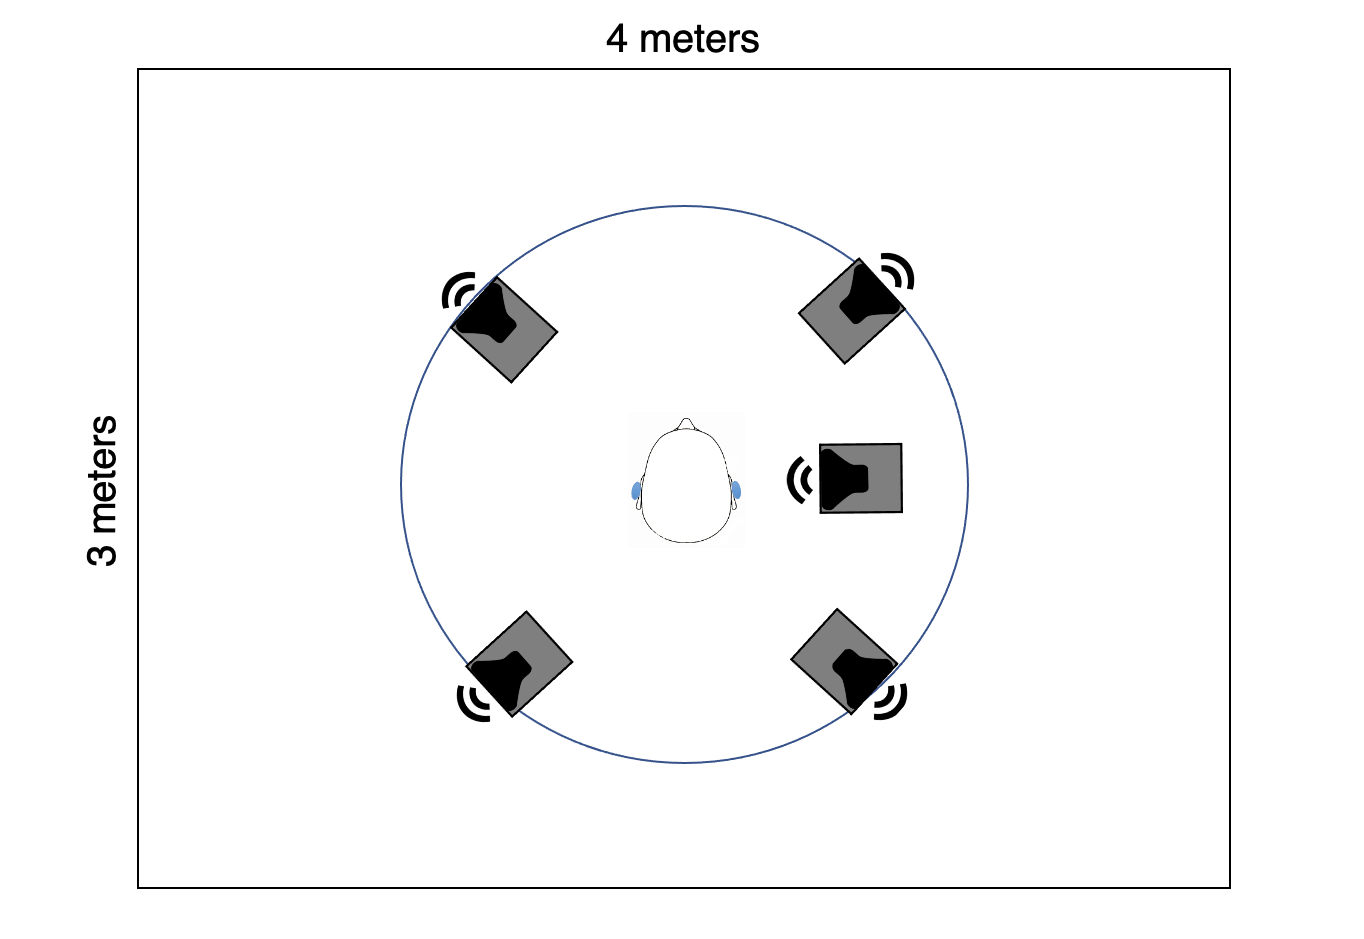}
\vskip -0.05in
\caption{\small{End-to-end system experiment physical set up. A foam mannequin head with a speaker (Sony SBS-XB12) inserted into its artificial mouth uttered one hundred VCTK samples from the test partition.
Ambient environmental sound (from WHAM! dataset) was played via four monitors (PreSonus Eris E3.5) positioned to fill 3 meter by 4 meter room on a 0.75 meter radius circle, and background voice (also VCTK) was played from a monitor positioned 0.4 meters from head on the right.}}
\label{fig:network}
\vskip -0.25in
\end{figure}
